# Supplementary material for: Tailoring the opto-electronic response of graphene nanoflakes by size and shape optimization
Source: arXiv:2003.02010 ancillary file (2020-03-04)
Supplement: Supplementary file 1 [file supplementary.pdf]

# Supplementary information for Tailoring the opto-electronic response of graphene nanoflakes by size and shape optimization

Raquel Esteban-Puyuelo[1], Rajat Kumar Sonkar[2], Bhalchandra Pujari[2], Oscar Grånäs[1], and Biplab Sanyal[1]

[1]Division of Materials Theory, Department of Physics and Astronomy, Uppsala University, Box-516, SE 75120, Sweden

[2]Centre for Modeling and Simulation, Savitribai Phule Pune University, Ganeshkhind, Pune 411007, India

## 1 Computational details

The main code used in our study is Siesta [1]. We have used a triple-zeta + double polarization basis set to calculate ground and excited state properties. The real-time *ab-initio* approach used here is based on TD-DFT, as implemented in the TDAP package [2], built on top of the Siesta code. We propagate the electronic density according to the time-dependent Kohn-Sham (TD-KS) equations:

$$i\hbar \frac{\partial \phi_n(\boldsymbol{r},t)}{\partial t} = \mathcal{H}_{\mathrm{KS}}[\rho]\phi_n(\boldsymbol{r},t), \tag{1}$$

with

$$\mathcal{H}_{\mathrm{KS}}[\rho] = -\frac{\hbar^2}{2m}\nabla_{\boldsymbol{r}}^2 + v_{\mathrm{ext}} + \int \frac{\rho(\boldsymbol{r}',t)}{|\boldsymbol{r}-\boldsymbol{r}'|} - \sum \frac{Z_N}{|\boldsymbol{r}-\boldsymbol{R}_j|} + v_{\mathrm{xc}}[\rho](t) \tag{2}$$

where $\phi_n$ are the single electron KS wave functions, $v_{\mathrm{ext}}$ is the external potential, $v_{\mathrm{xc}}$ is the exchange-correlation potential and the electronic density is

$$\rho(\boldsymbol{r},t) = \sum_{n=1}^{N} |\phi_n(\boldsymbol{r},t)|^2, \tag{3}$$

where the sum runs over the number of electrons $N$. This means that the electronic subsystem is only dependent on its initial state.

An iterative solution of eq 1 is given by

$$\phi_n(t) = \mathcal{U}(t,t_0)\phi_n(t_0) = \hat{T}\exp\left(-i\hbar\int_{t_0}^{t}\mathcal{H}_{\mathrm{KS}}(t')dt'\right), \tag{4}$$

where the wave functions are known at an initial time $t_0$, $\mathcal{U}$ is the time-evolution operator and $\hat{T}$ is the time-ordering operator. In TDAP $\mathcal{U}$ is approximated with the second-order Magnus expansion:

$$\mathcal{U}(t+\Delta t,t) \approx \left[-i\hbar\Delta t\mathcal{H}_{\mathrm{KS}}\left(t+\frac{\Delta t}{2}\right)\right] \tag{5}$$

for a finite time step $\Delta t$.

The Hamiltonian matrices and wave functions at each time step are computed. The calculations use a local basis comprising a set of numerical atomic orbitals built from atomic pseudopotentials. This provides a finite and orthonormal basis set, which lets us approximate the TD-KS to

$$i\hbar\frac{\partial \boldsymbol{c}}{\partial t} = \boldsymbol{S}^{-1}(\mathcal{H} - i\hbar\boldsymbol{P}), \tag{6}$$

with $c$ being a column vector containing the basis coefficients, $\boldsymbol{S}$ the overlap matrix and $\boldsymbol{P}$ is a matrix that appears due to the motion of the basis functions. Eq 5 is approximated by evaluating the matrices at the half time step:

$$\mathcal{U}(t+\Delta t,t) \approx \left\{-i\hbar\Delta t\left[\boldsymbol{S}_{1/2}^{-1}\left(\mathcal{H}_{1/2} - i\hbar\boldsymbol{P}_{1/2}\right)\right]\right\}. \tag{7}$$

We have also used Octopus and NWChem codes to calculate the electronic structure and optical absorption spectra in our validation simulations using TD-DFT. Octopus is a pseudopotential real-space package to perform TD-DFT calculations [3, 4]. The time-dependent Kohn-Sham (TDKS) orbitals are expanded in a regular mesh in real space, and the simulations are performed in real time. The NWChem code [5] utilizes Gaussian basis sets. The "Enforced Time-Reversal Symmetry (ETRS)" propagator has been used in the real-time TD-DFT implementation.

## 2 Auxilliary rectangular geometries

In this section we present results pertaining to structures with broken symmetry, specifically 16×6 and 17×5 RGNFs. The broken symmetry results in undercoordinated carbon atoms on the edge of the flake. With respect to the 17×6-RGNF, the 16×6-RGNF correspond to the removal of a vertical dimer line, and the 17×5-RGNF the removal of a zigzag line. Figure 1 shows their FM and AFM magnetization densities. Despite the symmetry break, the general features of the magnetization density is maintained. Similarly to the 17×6-RGNF, the same competition between frustration in the center in the FM structure against magnetization in the armchair edges in the AFM structure applies.

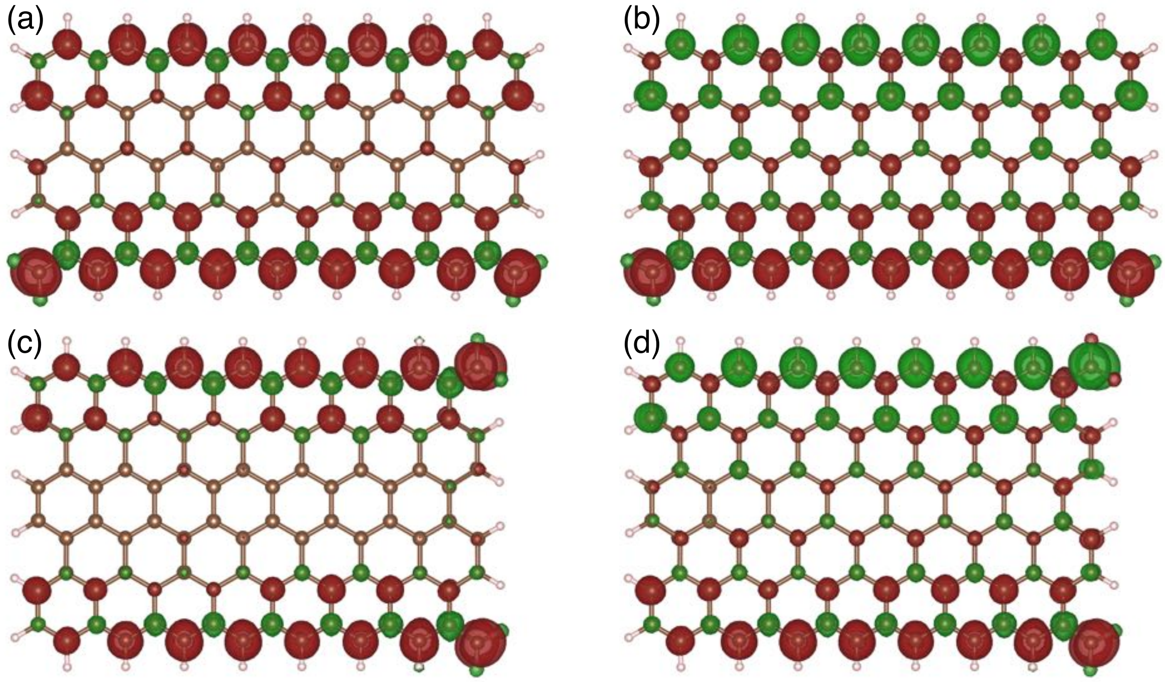


Figure 1: Magnetization densities of variations of the rectangular flake. The red (green) color represents positive (negative) values. The FM (a) and AFM (b) of a 17×5-RGNF solutions differ by 1.2 meV/atom, while the FM (c) and AFM (d) solutions of a 16×6 flake differ only by 0.37 meV/atom, which is comparable to the original difference on the 17×6-RGNF in Figure 1.

The coupling between the zigzag edges becomes stronger when the flake is narrower as in 17×5-RGNF and the AFM solution is more favourable by 1.2 meV/atom, which is larger than the 0.5 meV/atom of the original 17×6-RGNF. On the contrary, 16×6-RGNF has the same distance between the zigzag edges as the original flake, but armchair edges are closer. This seems not to have an appreciable effect, as the AFM-FM energy difference is 0.37 meV/atom in this case, comparable to 17×6-RGNF. We also studied flakes in which we removed alternating atoms of the zigzag edge so that the horizontal edge is no longer zigzag. Breaking the zigzag pattern makes the modified edge loose the magnetization. This points toward the necessity of zigzag edges for realizing magnetism, similar to what can be expected based on experience with GNR [6].

We also present the bond-lengths of the edge carbon atoms of the 17x$N_z$ flakes, with $N_z \in \{2, 4, 6, 8\}$. The 17×2 flake is a polyacene, similar to what is studied by e.g. Hachmann and co-workers [7]. We see that the FM vs AFM solution for the polyacene shows a clear difference in bond-length, similar to what Qu and co-workers see when comparing singlet and triplet solutions. Additionally, it is clear that as the number of armchair edges increase (increased distance between the spin-carrying zigzag edge), the FM and AFM becomes more equal. This is a natural effect of the decreased overlap between the wave-functions, in turn leading to the decreased exchange coupling.

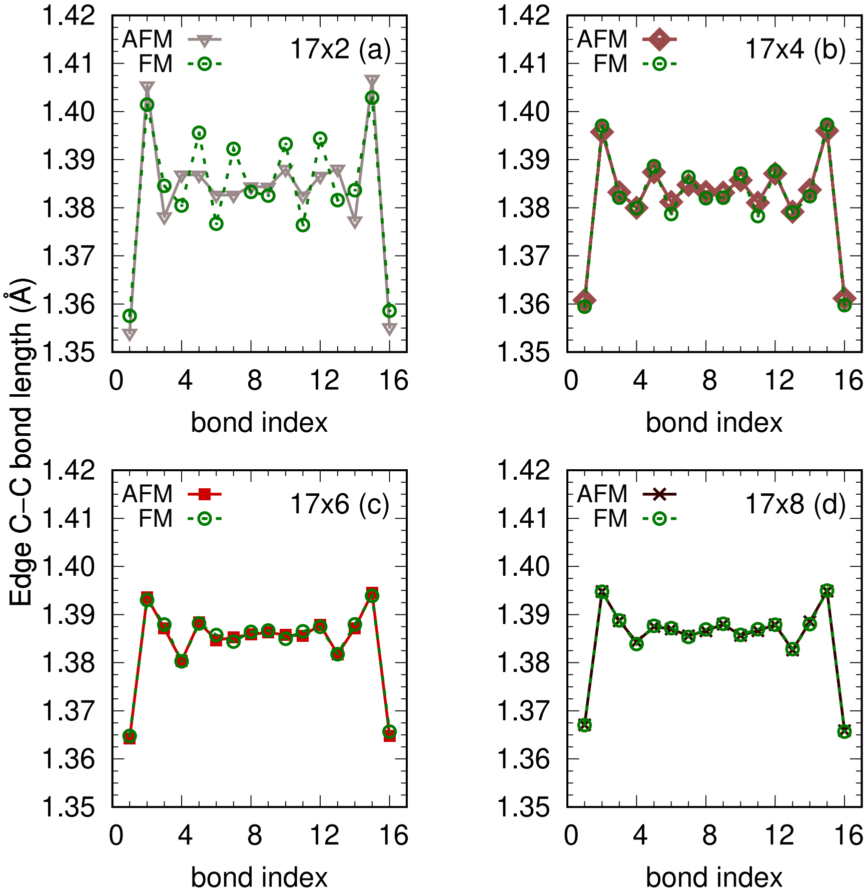


Figure 2: Carbon-carbon bond-lengths along the lower zigzag edges of RGNFs.

# 3 Rhomboid flakes

We present the results of a rhomboid flake with zigzag edges (Figure 3). We considered four initial magnetic configurations depending on the coupling between zigzag edges. Only the ferromagnetic (FM) and one of the antiferromagnetic ($AFM_1$) structures could be stabilized as magnetic solutions. $AFM_1$ has a lower energy than FM by 0.98 meV/atom. The magnetic moments on the superior and inferior edges are of the order of the zigzag edges in the RGNF. Similarly, the FM has a central frustration and the magnetic moments are quenched, which is not the case in the $AFM_1$ configuration.

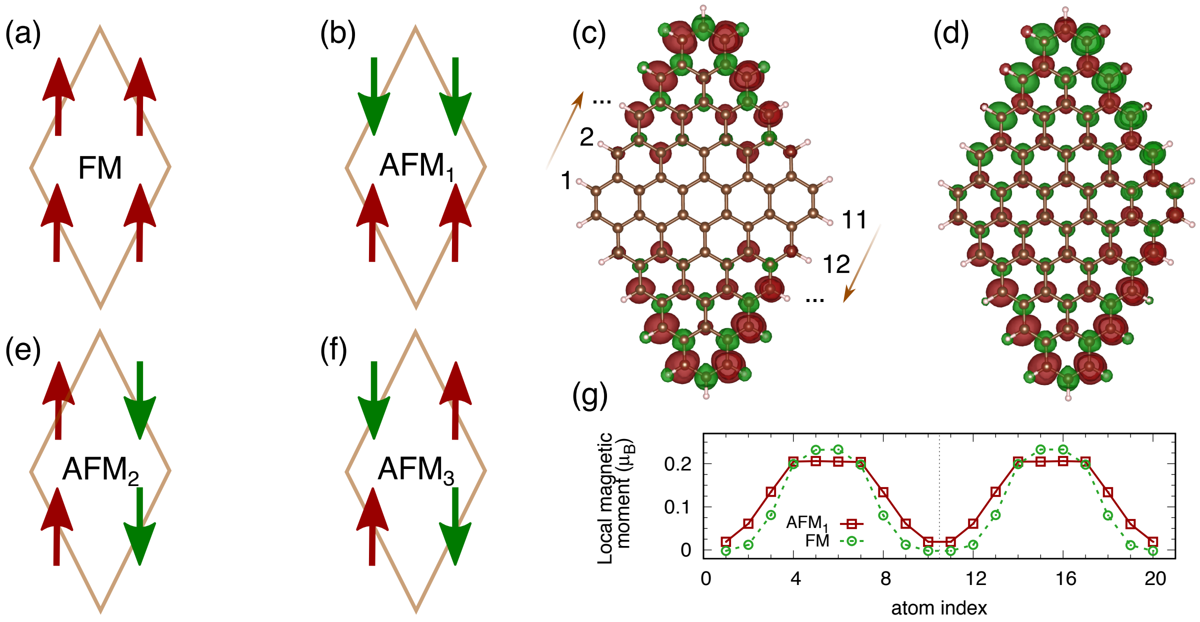


Figure 3: Rhomboid graphene nanoflake. The considered magnetic configurations are ferromagnetic (FM) shown in (a), and three different antiferromagnetic configurations: $AFM_1$ (b), $AFM_2$ (e) and $AFM_3$ (f). The magnetisation densities of FM and $AFM_1$ are shown in (c) and (d), and the local magnetic moments of the edge atoms are included in (g). The atom index is represented in (c).

# 4 Validation simulations

In addition to the results presented in the main text, we validate aspects of our findings by different codes, in particular for the optical absorption. Ground state properties were recently compared extensively by Lejaeghere et al. [8]. While our benchmark indicates that trends are similar in the results obtained from all codes, the quantitative differences seen for excited state properties for different basis sets call for similar undertakings as Lejaegere et al. has performed, but for excited state properties.

The three codes used for the benchmark provided here have different types of basis functions. The Octopus code uses a real-space grid to represent the wave-functions. NWChem and Siesta/TDAP use atom-centered basis function, Gaussian-type orbitals (GTO) and Numerical Atom-centered Orbitals (NAO) respectively. The grid allows for an unbiased description of the wave-function with respect to the atomic position, as the sampling is equally dense away from the nuclei. On the other hand, it is harder to converge the grid close to the nucleus, rendering tightly-bound states more difficult to calculate accurately with an equidistant grid than with NAOs or GTOs. For the latter two bases types, it is known that high-energy states are sometimes hard to resolve if not additional diffuse basis functions are added. Hence, the three approaches used have positive and negative traits for different parts of the electronic-structure, the tightly bound and the weakly bound states. In our simulation, we have a more diffuse basis for the Siesta calculations than for the NWChem calculations. We expect that this has implications, primarily on the absorption strength, for the outcome of our calculated absorption spectra. We elaborate on this fact in the sections below. For this benchmark, we have considered reasonably small molecules as benzene, naphtalene, flourene and coronene.

Fig 4 shows the optical spectra of benzene, naphthalene, fluorene and coronene obtained from Octopus, NWChem and TDAP codes. The three codes qualitatively agree regarding the positions of the peaks, specially at low energies. Furthermore, Octopus derived peaks appear at slightly lower energies followed by those obtained from TDAP and then NWChem at higher energies. This tendency is maintained throughout the energy range for the four studied molecules, and it can be clearly seen in Table 1, which contains information about the position of the first peak in the optical spectra of the four molecules depending on the code, as well as a comparison with the Kohn-Sham HOMO-LUMO gap for the TDAP calculations.

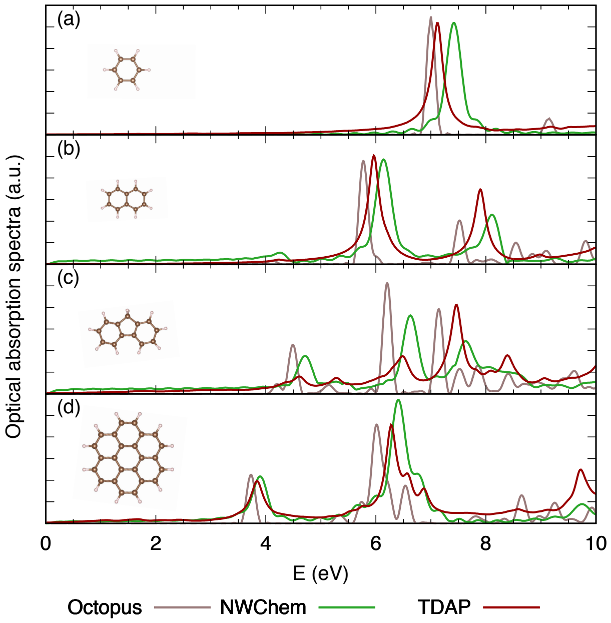


Figure 4: Comparison of optical spectra obtained from Octopus, NWChem and TDAP for benzene (a), naphthalene (b), fluorene (c) and coronene (d). Interestingly, the peak-positions correlate well with the degree of diffuseness of the basis, with a lower absorption energy for the more diffuse basis.

The optical absorption spectrum in benzene has its first peak at rather high energies compared with the rest of the molecules, followed by fluorene, naphtalene and then coronene. One would expect that the first peak would appear at lower energies with increasing size, but fluorene is an exception. Figure 5 shows the wave-functions for the HOMO-1, HOMO, LUMO and LUMO+1 energy levels of the studied molecules calculated with Siesta. Although the optical absorption spectrum in TDAP is obtained from RT-TDDFT, the symmetries of the ground state wave-functions can help us to understand the first peak positions.

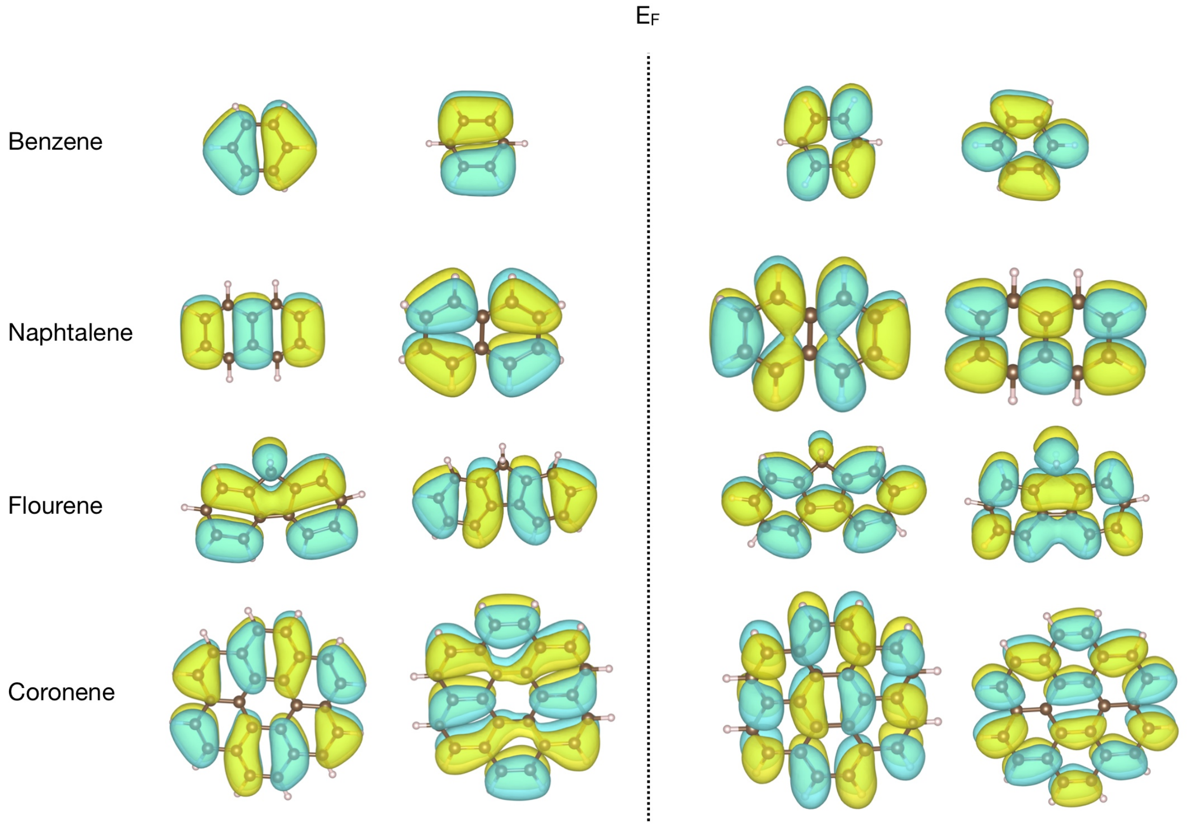


Figure 5: Wave-functions for HOMO-1, HOMO, LUMO and LUMO+1 of the respective small molecules (yellow and blue represent positive and negative lobes respectively). For benzene and coronene, the HOMO levels are degenerate, in the case of benzene also the two LUMO levels are degenerate. The higher HOMO-LUMO gap in Naphtalene, and corresponding higher absorption threshold than fluorene is explained by the decreased ability to form conjugated bonds with the lower symmetry structure.

Table 1: Position of the first peak in the optical spectra calculated with NWChem, Octopus and TDAP. The HOMO-LUMO gap as calculated by TDAP is specified in parentheses. Units are in eV.

| Method | Benzene | Naphthalene | Fluorene | Coronene |
|---|---|---|---|---|
| NWChem | 7.45(5.48) | 4.27(3.6) | 4.71(3.86) | 3.95(3.03) |
| Octopus | 7.00 | 4.12 | 4.20 | 3.70 |
| TDAP | 7.12 (5.36) | 4.23 (3.52) | 4.60 (3.78) | 3.84 (2.98) |
| Experiments | 6.97 [9] | 4.75 [10] | 4.12 [11] | 3.28 [12] |

# References


[1] J. M. Soler, E. Artacho, J. D. Gale, A. García, J. Junquera, P. Ordejón, and D. Sánchez-Portal, "The SIESTA method for ab initio order-N materials simulation," *Journal of Physics: Condensed Matter J. Phys.: Condens. Matter*, vol. 14, pp. 2745–2779, 2002.

[2] G. Kolesov, O. Grånäs, R. Hoyt, D. Vinichenko, and E. Kaxiras, "Real-Time TD-DFT with Classical Ion Dynamics: Methodology and Applications," *Journal of Chemical Theory and Computation*, vol. 12, no. 2, pp. 466–476, 2016.

[3] M. A. Marques, A. Castro, G. F. Bertsch, and A. Rubio, "Octopus: A first-principles tool for excited electron-ion dynamics," *Computer Physics Communications*, vol. 151, pp. 60–78, mar 2003.

[4] A. Castro, H. Appel, M. Oliveira, C. A. Rozzi, X. Andrade, F. Lorenzen, M. A. Marques, E. K. Gross, and A. Rubio, "Octopus: A tool for the application of time-dependent density functional theory," *Physica Status Solidi (B) Basic Research*, vol. 243, pp. 2465–2488, sep 2006.

[5] M. Valiev, E. J. Bylaska, N. Govind, K. Kowalski, T. P. Straatsma, H. J. Van Dam, D. Wang, J. Nieplocha, E. Apra, T. L. Windus, and W. A. De Jong, "NWChem: A comprehensive and scalable open-source solution for large scale molecular simulations," *Computer Physics Communications*, vol. 181, pp. 1477–1489, sep 2010.

[6] Y.-W. Son, M. L. Cohen, and S. G. Louie, "Energy Gaps in Graphene Nanoribbons," *Physical Review Letters*, vol. 97, p. 216803, nov 2006.

[7] Z. Qu, D. Zhang, C. Liu, and Y. Jiang, "Open-Shell Ground State of Polyacenes: A Valence Bond Study," *J. Phys. Chem. A*, vol. 113, no. 27, pp. 7909–7914, 2009.

[8] K. Lejaeghere, G. Bihlmayer, T. Björkman, P. Blaha, S. Blügel, V. Blum, D. Caliste, I. E. Castelli, S. J. Clark, A. Dal Corso, S. de Gironcoli, T. Deutsch, J. K. Dewhurst, I. Di Marco, C. Draxl, M. Dułak, O. Eriksson, J. A. Flores-Livas, K. F. Garrity, L. Genovese, P. Giannozzi, M. Giantomassi, S. Goedecker, X. Gonze, O. Grånäs, E. K. U. Gross, A. Gulans, F. Gygi, D. R. Hamann, P. J. Hasnip, N. A. W. Holzwarth, D. Iuşan, D. B. Jochym, F. Jollet, D. Jones, G. Kresse, K. Koepernik, E. Küçükbenli, Y. O. Kvashnin, I. L. M. Locht, S. Lubeck, M. Marsman, N. Marzari, U. Nitzsche, L. Nordström, T. Ozaki, L. Paulatto, C. J. Pickard, W. Poelmans, M. I. J. Probert, K. Refson, M. Richter, G.-M. Rignanese, S. Saha, M. Scheffler, M. Schlipf, K. Schwarz, S. Sharma, F. Tavazza, P. Thunström, A. Tkatchenko, M. Torrent, D. Vanderbilt, M. J. van Setten, V. Van Speybroeck, J. M. Wills, J. R. Yates, G.-X. Zhang, and S. Cottenier, "Reproducibility in density functional theory calculations of solids," *Science*, vol. 351, no. 6280, 2016.

[9] J. Romand and B. Vodar, "Spectres d'absorption du benzene a l'etat vapeur et a l'etat condense dans l'ultraviolet lointain," *Comptes rendus de l'Académie des Sciences*, vol. 233, no. 17, pp. 930–932, 1951.

[10] J. Ferguson, L. W. Reeves, and W. G. Schneider, "Vapor absorption spectra and oscillator strengths of naphthalene, anthracene, and pyrene," *Canadian Journal of Chemistry*, vol. 35, no. 10, pp. 1117–1136, 1957.

[11] M. Ramart-Lucas, M. J. Matti, and T. Guilmart, "Structure, absorption et comportement chimique dans la serie du phenanthrene," *Bulletin de la Societe Chimique de France*, vol. 15, no. 11-1, pp. 1215–1224, 1948.

[12] P. G. Schroeder, C. B. France, B. A. Parkinson, and R. Schlaf, "Orbital alignment at p-sexiphenyl and coronene/layered materials interfaces measured with photoemission spectroscopy," *Journal of applied physics*, vol. 91, no. 11, pp. 9095–9107, 2002.
